# Supplementary material for: On the Integration of Battery Electric Buses into Urban Bus Networks
Source: arXiv:2103.12189 source file (2021-03-22)
Supplement: Supplementary file 1 [file appendix-B.tex]

\section{Objective function}\label{apx:B}
In addition to the notation from Section~\ref{sect:model} as summarized in Table~\ref{tab:notation_appendix}, we denote with $C_{t}^{\text{bm}}$ the costs for bus maintenance in period $t$ and with $C_{t}^{\text{en}}$ the costs for fuel or electricity in period $t$. Then the single terms of the objective result as follows.
Besides considering costs for the initial bus fleet composition, the costs associated with the bus fleet transformation consist of costs for purchasing new buses and replacing batteries~(\ref{eq:C_b}) minus salvage revenues that occur at the end of the holding periods of buses~(\ref{eq:V_b}). \ndmargin{The costs for purchasing includes costs for buses, new batteries as well as battery replacement costs. The salvage revenue is calculated by linear depreciation and a salvage value for the bus but not for the battery. However,}{New.} at the end of the planning horizon, a payment~(\ref{eq:V_b_n}) equal to the total final salvage value of all buses~(\ref{eq:V_d}) and batteries~(\ref{eq:V_q}) \ndmargin{based on linear depreciation}{New.} is taken into account. Costs for charging infrastructure consist of installation and maintenance costs~(\ref{eq:C_f}). \ndmargin{For this purpose the number of newly installed charging stations is monitored in each period.}{New.} Finally, operational costs~(\ref{eq:C_o}) are due to maintenance and repair of the bus fleet~(\ref{eq:C_bm}) as well as energy consumption depending on total distance covered~(\ref{eq:C_e}). \ndmargin{Herein, service trips and deadheading trips are considered. In contrast to the maintenance costs, the energy costs depend on whether passengers are transported (service trip) or not (deadheading trip).}{New.}
\begin{table}[!hb]
	\centering
	\setlength{\abovecaptionskip}{0.5ex}
	\addtolength{\tabcolsep}{-3pt}			
	\caption{Notation of cost terms.}
	\label{tab:notation_appendix}
	\footnotesize
	\begin{tabular}{rl} 					
		\toprule
		$C_{t}^{\text{b}}$			
		& costs for purchasing buses in period $t$\\ 	
		$V_{t}^{\text{b}}$			
		& revenue due to selling buses in period $t$\\ 			
		$V_{t_{\text{n}+1}}^{\text{b}}$
		& final bus fleet salvage value\\
		$C_{t}^{\text{f}}$ &
		costs for charging facility installations and maintenance in period $t$\\ 
		$C_{t}^{\text{o}}$
		& operational costs in period $t$\\
		\bottomrule
	\end{tabular}				
\end{table}
% 02 --------------------------------------------------------
%\vspace{-1cm}
{
	\setlength{\abovedisplayskip}{3pt}
	\setlength{\abovedisplayshortskip}{3pt}
	\setlength{\belowdisplayskip}{3pt}
	\setlength{\belowdisplayshortskip}{3pt}
\begin{multline}
	\quad\quad\quad
	C_{t}^{\text{b}} =
	\sum_{k \in \mathcal{K}} c_{k}^{\text{b}} p_{kt} + \sum_{k \in \mathcal{K}^{\text{BEB}}} c_{kt}^{\text{q}} Q_{k} \left( p_{kt}+p_{k,t-e^{\text{q}}} \right)
	\hfill \forall t \in \mathcal{T}
	\label{eq:C_b}
\end{multline}
% 03 --------------------------------------------------------
%\vspace{-1cm}
\begin{multline}
	\quad\quad\quad
	V_{t}^{\text{b}}=
	\sum_{k \in \mathcal{K}} \left( \left( c_{k}^{\text{b}} - v^{\text{b}} \right)\left( 1 - \frac{h_{k}}{e^{\text{b}}} \right) + v^{\text{b}} \right) p_{k,t-h_{k}}
	\hfill \forall t \in \mathcal{T}
	\label{eq:V_b}
\end{multline}
% 04 --------------------------------------------------------
%\vspace{-1cm}
\begin{multline}
	\quad\quad\quad
	V_{t_{\text{n+1}}}^{\text{b}} =
	\sum_{k \in \mathcal{K}}
	V_{kt_{\text{n+1}}}^{\text{d}} +
	\sum_{k \in \mathcal{K}^{\text{BEB}}} V_{kt_{\text{n+1}}}^{\text{q}}
	\hfill
	\label{eq:V_b_n}
\end{multline}
% 05 --------------------------------------------------------
%\vspace{-1cm}
\begin{multline}
	\quad\quad\quad
	V_{kt_{\text{n+1}}}^{\text{d}} =
	\sum_{t \in \lbrace \mathcal{T}\,|\,t \geq t_{\text{n}+1} - h_{k} \rbrace}
	\left( \left( c_{k}^{\text{b}} - v^{\text{b}}\right) \left( 1 - \frac{t_{\text{n+1}}-t}{e^{\text{b}}} \right) + v^{\text{b}} \right) p_{kt}
	\\
	\hfill \forall k \in \mathcal{K}
	\label{eq:V_d}
\end{multline}
% 06 --------------------------------------------------------
%\vspace{-1cm}
\begin{multline}
	\quad\quad\quad
	V_{kt_{\text{n+1}}}^{\text{q}} =
	\sum_{t \in \lbrace \mathcal{T}\,|\,t \geq t_{\text{n+1}} - e^{\text{q}} \rbrace}
	c_{kt}^{\text{q}} Q_{k} \left( 1 - \frac{t_{\text{n+1}}-t}{e^{\text{q}}} \right) (p_{kt}+p_{k,t-e^{\text{q}}})
	\\
	\hfill \forall k \in \mathcal{K}^{\text{BEB}}
	\label{eq:V_q}
\end{multline}
% 07 --------------------------------------------------------
%\vspace{-1cm}
\begin{multline}
	\quad\quad\quad
	C_{t}^{\text{f}} = \sum_{i \in \mathcal{R}} \left(  c^{\text{n}} (y_{it} - y_{i,t-1}) + c^{\text{nm}} y_{it} \right)
	+ c^{\text{d}}(a_{t}-a_{t-1})+c^{\text{dm}}a_{t}
	\\
	\hfill \forall t \in \mathcal{T}
	\label{eq:C_f}
\end{multline}
% 08 --------------------------------------------------------
%\vspace{-1cm}
\begin{multline}
	\quad\quad\quad
	C_{t}^{\text{o}} = \eta \left( C_{t}^{\text{bm}} + C_{t}^{\text{e}} \right)
	\hfill \forall t \in \mathcal{T}
	\label{eq:C_o}
\end{multline}
% 09 --------------------------------------------------------
%\vspace{-1cm}
\begin{multline}
	\quad\quad\quad
	C_{t}^{\text{bm}} = 
	\sum_{k \in \mathcal{K}}\sum_{s \in \mathcal{S}} c_{k}^{\text{bm}}
	\left(
	\sum_{i \in \mathcal{N}_{s}}l_{i} +
	\sum_{(i,j) \in \mathcal{A}_{s}}d_{ij}
	\right)
	x_{skt}
	\hfill \forall t \in \mathcal{T}
	\label{eq:C_bm}
\end{multline}
% 10 --------------------------------------------------------
%\vspace{-1cm}
\begin{multline}
	\quad\quad\quad
	C_{t}^{\text{e}} = \sum_{k \in \mathcal{K}}\sum_{s \in \mathcal{S}}
	c_{k}^{\text{e}} \left(
	o_{k}^{\text{p}} \sum_{i \in \mathcal{N}_{s}}l_{i} +
	o_{k}^{\text{e}} \sum_{(i,j) \in \mathcal{A}_{s}}d_{ij}
	\right)
	x_{skt}
	\hfill \forall t \in \mathcal{T}
	\label{eq:C_e}
\end{multline}
}
